# Supplementary material for: MT4CrossOIE: Multi-stage Tuning for Cross-lingual Open Information Extraction
Source: arXiv:2308.06552 source file (2023-09-20)
Supplement: Supplementary file 1 [file appendix.tex]

\appendix
\section{Statistics of Datasets}

\section{Details}

% \bibliography{custom}
% \bibliographystyle{acl_natbib}
% \end{document}
